# Supplementary material for: Design of Robust and Efficient Edge Server Placement and Server Scheduling Policies: Extended Version
Source: arXiv:2104.14256 source file (2021-04-29)
Supplement: Supplementary file 1 [file Appendix1.tex]

\section{Single-Gigantic-OCS Abstraction}\label{Appendix1}
Consider an arbitrary PoD-level topology $X=[x_{ij},i,j=1,...,n]$ satisfying (\ref{Toe:valid}). If there were only one gigantic OCS, we can easily realize the topology $X$ using this gigantic OCS. Hence, in order to prove that our multi-OCS physical structure is equivalent to a single gigantic OCS structure, we need to prove that the topology $X$ is also realizable in our multi-OCS physical structure.

In order to prove this statement, we need the following lemma. (Lemma \ref{IntegerDecomposition} is a direct consequence of Theorem 3 in \cite{zhao2018minimalextended}, by setting $\mathcal{A}=\mathcal{B}=\{\{1\}, \{2\},...,\{n\}\}$.)
\begin{lemma}\label{IntegerDecomposition}
Given an $n\times n$ non-negative integer matrix $X=[x_{ij},i,j=1,...,n]$ and an integer $K\geq 1$, there exist $K$ integer matrices $X^{(k)}=[x_{ij}^{(k)},i,j=1,...,n], k=1,2,...,K$ satisfying
\begin{enumerate}
    \item for any $i=1,2,...,n$ and $j=1,2,...,n,$ $$x_{ij}=x_{ij}^{(1)}+x_{ij}^{(2)}+\cdots+x_{ij}^{(K)}$$
    \item for any $i=1,2,...,n, j=1,2,...,n$ and $k=1,2,...,K$, $$\left\lfloor\frac{x_{ij}}{K}\right\rfloor\leq x_{ij}^{(k)}\leq \left\lceil\frac{x_{ij}}{K}\right\rceil$$
    \item for any $j=1,2,...,n$ and $k=1,2,...,K$, $$\left\lfloor\frac{\sum_{i=1}^n x_{ij}}{K}\right\rfloor\leq \sum_{i=1}^n x_{ij}^{(k)}\leq \left\lceil\frac{\sum_{i=1}^n x_{ij}}{K}\right\rceil$$
    \item for any $i=1,2,...,n$ and $k=1,2,...,K$, $$\left\lfloor\frac{\sum_{j=1}^n x_{ij}}{K}\right\rfloor\leq \sum_{j=1}^n x_{ij}^{(k)}\leq \left\lceil\frac{\sum_{j=1}^n x_{ij}}{K}\right\rceil$$
\end{enumerate}
\end{lemma}

Assume that there are $K$ OCSs in the DCN core layer. In our multi-OCS physical structure, the uplinks of each PoD are evenly connected to the $K$ OCSs. Hence, the total number of links between PoD $i$ and each OCS is exactly $\frac{r_i}{K}$. According to Lemma \ref{IntegerDecomposition}, the PoD-level topology $X$ can be decomposed into $K$ sub-topologies satisfying the four constraints in Lemma \ref{IntegerDecomposition}. According to the third and the fourth constraints in Lemma \ref{IntegerDecomposition}, each sub-topology $X^{(k)}$ must satisfy
\begin{equation}\label{eqn:each_ocs_constraint}
\left\{\begin{array}{l}
\sum_{j=1}^n x_{ij}^{(k)}\leq \left\lceil\frac{\sum_{j=1}^n x_{ij}}{K}\right\rceil \leq \frac{r_i}{K},\forall i=1,...,n,\\
\sum_{i=1}^n x_{ij}^{(k)}\leq \left\lceil\frac{\sum_{i=1}^n x_{ij}}{K}\right\rceil \leq \frac{r_j}{K}, \forall j=1,...,n.\\
\end{array}\right.
\end{equation}
Equation (\ref{eqn:each_ocs_constraint}) indicates that the sub-topology $X^{(k)}$ is realizable on the $k$-th OCS. Hence, we can realize the topology $X$ in our multi-OCS physical structure.
